# Supplementary material for: Mapping the Multilingual Margins: Intersectional Biases of Sentiment Analysis Systems in English, Spanish, and Arabic
Source: arXiv:2204.03558 source file (2022-04-07)
Supplement: Supplementary file 1 [file appendix_template.tex]

% \setarab % choose the language specific conventions
% \vocalize % switch diacritics for short vowels on
%\transtrue % display the transliteration
% \arabtrue % print arabic text (on by default)
% \usepackage{utf8}
% \setcode{utf8}

\begin{table*}[t]
\centering
\scalebox{0.8}{
\begin{tabular}{| l | }
\hline
Sentence Template\\
\hline
\begin{tabular}[t]{@{}l@{}}[p] feels [eA]\end{tabular}\\
\begin{tabular}[t]{@{}l@{}}The situation makes [p] feel [eA]\end{tabular}\\
\begin{tabular}[t]{@{}l@{}}I made [p] feel [eA]\end{tabular}\\
\begin{tabular}[t]{@{}l@{}}[p] made me feel [eA]\end{tabular}\\
\begin{tabular}[t]{@{}l@{}}[p] found himself/herself in a/an [eB] situation\end{tabular}\\
\begin{tabular}[t]{@{}l@{}}[p] told us all about the recent [eB] events\end{tabular}\\
\begin{tabular}[t]{@{}l@{}}The conversation with [p] was [eB]\end{tabular}\\
\begin{tabular}[t]{@{}l@{}}I saw [p] in the market\end{tabular}\\
\begin{tabular}[t]{@{}l@{}}I talked to [p] yesterday\end{tabular}\\
\begin{tabular}[t]{@{}l@{}}[p] goes to the school in our neighborhood\end{tabular}\\
\begin{tabular}[t]{@{}l@{}}[p] has two children\end{tabular}\\
\hline
\end{tabular}
}
\caption{Sentence templates used in the EECs}
\label{tab:eectemplates}
\end{table*}
